# Supplementary material for: Conceptualization of seeded region growing by pixels aggregation. Part 4: Simple, generic and robust extraction of grains in granular materials obtained by X-ray tomography
Source: arXiv:0806.3939 source file (2008-07-23)
Supplement: Supplementary file 1 [file appendice.tex]

\appendices
\section{Problem if not component by component}
